# Supplementary material for: Composing Text and Image for Image Retrieval - An Empirical Odyssey
Source: arXiv:1812.07119 source file (2018-12-18)
Supplement: Supplementary file 1 [file appendix.tex]

\section{Identity connection}

The difference between our proposed approach compared to baseline such as concat fusion is having the identity connection contributing to the output feature.
In section 4.2, we show some visualizations to demonstrate the effect of having an identity connection. On the MIT-State dataset, we can show some quantitative effect. Here the retrieved image is considered correct if it has the correct object label (extracted from the image part of the query) and the correct state label (extracted from the text part of the query). Hence in addition to measuring composition retrieval performance, we can also measure correct object or correct state retrieval performance to analyze how well the composition module extract those separate information from each channel of the input query, the result is shown in figure \ref{fig:mitstates_r1_object_state}.

For the concat fusion (and also other baselines that creates new output feature from input), the object, state and together composition performance improves during training as expected. Differently, for our approach, the object retrieval performance is already quite high right at the beginning. This is because the output feature is mostly the query image feature with no modification is yet learned. As training goes, correct object performance is actually compromised to improve the overall correct composition retrieval performance.

We can measure the contribution to the composition feature of the identity connection by computing its magnitude over the sum of all connection's magnitude. It'd start big and then get smaller as the residual connection learns to model the needed modification. In table \ref{tab:identity}, we show that value for each dataset when training converged. It seems that with more realistic images and complex composition, Fashion200k and MIT-States are relying less on the identity connection compared to CSS.

\begin{figure*}
\begin{center}
\includegraphics[width=0.9\linewidth]{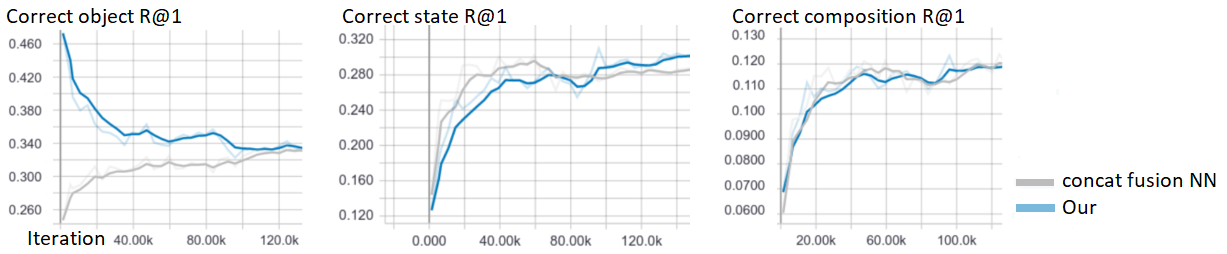}
\end{center}
   \caption{Retrieval performance changing during training on MIT-States.}
\label{fig:mitstates_r1_object_state}
\end{figure*}

\begin{table}
\begin{center}
\begin{tabular}{|l|c|}
\hline
Dataset & Identity's contribution \\
\hline\hline
CSS & 62\% \\
Fashion200k  & 20\% \\
MIT-States & 31\% \\
\hline
\end{tabular}
\end{center}
\caption{The average contribution to the composition feature of the identity connection in our approach in each dataset.}
\label{tab:identity}
\end{table}
