# Supplementary material for: Composing Text and Image for Image Retrieval - An Empirical Odyssey
Source: arXiv:1812.07119 source file (2018-12-18)
Supplement: Supplementary file 2 [file appendix-old.tex]

\section{Motivating dataset for composition query image search}

We create a image retrieval with composition query dataset to demonstrate the use case where pure text or image query is not expressive enough. Inspired by \cite{johnson2017clevr}, images will be simple synthesized scene of 3 by 3 grid world, where each position is either empty or occupied by an object. Each object is specified with 3 attributes: color (8 different values), size (2 different values) and shape (3 different values); we name the dataset CSS. Given a specification of such scene, we then render it in 2 modes: 2D and 3D, some examples are shown in figure \ref{fig:css}.

\subsection{Scene modification}

We define 3 types of transformation/modification that can be applied to a scene, this facilitates the need to perform composition between a scene image and a modification described by text.

Add object modification: specify a new object that will be placed in the scene (its color, size, shape, position), if any of the attribute is not specified, its value will be randomly chosen. Example of this modification in the form of text: “add object”, “add red cube”, “add big red cube to middle-center”.

Remove object modification: specify object that will be removed from the scene, all object that match the specified attribute values will be removed. Example of this modification in the form of text: “remove yellow sphere”, “remove middle-center object”.

Change object modification: specify object that will be changed and the new attribute value. The new attribute value has to be either color or size. All objects that match the specified attribute will be changed. Example: “make yellow sphere small”, “make middle-center object red”.


\lu{draw some figure to analyze this dataset. We can do this after the deadline.}

\subsection{Dataset generation}

First, we generate 1k random scenes as the base, which will be used as query images. Then we randomly generate modifications and apply them to the base images, resulting in a set of around 16k target images. Note that one base image can be transformed to multiple/different target images, and one modification can be applied to multiple/different base images.

We obtain a set of around 17k images, with 16k query-target pairs for training. An example is shown in figure \ref{fig:task} (top row). The process is repeated to generate a test set; therefore there will be ~16k test queries and the retrieval database will be the whole test set of 17k images.

Finally when generating base images we follow Condition A in \cite{johnson2017clevr} for train set, and condition B for test set (certain object shape and color combination only appear in one condition and not the other). So the base scene in training and testing can be different and we can see if the system generalizes.


\begin{figure}[t]
\begin{center}
\includegraphics[width=0.7\linewidth]{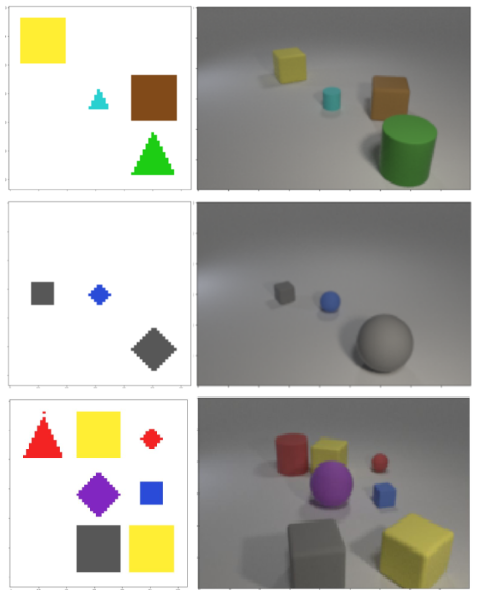}
\end{center}
   \caption{Example images in our CSS dataset. Each row shows the same scene in 2D and 3D rendered images.}
\label{fig:css}
\end{figure}


\section{Baseline methods}

Composing image and text is our main focus. This module takes the query as input, which includes a reference-image and a modification-text and output a feature vector representing the composition. Here we investigate some existing approaches, mostly from the area of vision and language joint understanding, and adapt them to our task.

One way is to perform feature extraction for each input (CNN for image and LSTM for text), then feature fusion using concatenation operation, followed by a feed forward network (2 layers in our implementation).
Concatenation is a very standard way to fuse features. This kind of composition has been used in VQA compositional reasoning, dialog-based image seach \cite{guo2018dialog}, attribute composition \cite{misra2017red} and attribute manipulation image search \cite{zhao2017memory}. While simple and straightforward, it has demonstrated very competitive performance.

Another approach is Show and Tell \cite{vinyals2015show}, well known for image captioning: the query image feature is first fed into a LSTM, and then followed by each of the word in the text, at each step the network predicts the next word. One can adapt it for this task by using the LSTM's last output as the image text composition feature.

Lastly, there's many image and text fusion techniques proposed for the VQA task. Some examples are parameter hashing \cite{noh2016image}, feature modulation FiLM \cite{perez2017film} and relationship network \cite{santoro2017simple}.




\begin{table}
\centering
\begin{tabular}{|l|ccc|}
\hline
Method & R@1 & R@5 & R@10 \\
\hline\hline
Image only & 3.3$^{\pm0.1}$ & 16.1$^{\pm0.2}$ & 27.7$^{\pm0.1}$ \\
Text only & 7.6$^{\pm0.4}$ & 27.9$^{\pm1.0}$ & 42.8$^{\pm0.8}$ \\
\hline
Concatenation & 11.8$^{\pm0.4}$ & 38.8$^{\pm0.6}$ & 54.6$^{\pm0.9}$ \\
Show and Tell & 11.9$^{\pm0.3}$ & 39.2$^{\pm0.5}$ & 55.0$^{\pm0.7}$ \\
Att. as Operator \cite{nagarajan2018attributes} & 8.9$^{\pm0.3}$ & 36.1$^{\pm0.2}$ & 52.7$^{\pm0.1}$ \\
Relationship \cite{santoro2017simple} & 12.3$^{\pm0.6}$ & 39.7$^{\pm0.7}$ & 54.9$^{\pm0.6}$ \\
FiLM \cite{perez2017film} & 10.9$^{\pm0.0}$ & 36.0$^{\pm0.0}$ & 53.7$^{\pm0.0}$ \\
Ours & 12.1$^{\pm0.4}$ & 40.4$^{\pm0.3}$ & 56.3$^{\pm0.4}$ \\
\hline
\end{tabular}
\caption{Retrieval performance on MIT-States.}
\label{tab:mitstates}
\end{table}


\section{MITStates}

We create an image retrieval benchmark using this dataset as following: pairs of images with the same object labels and different state labeled are sampled. They are using as query image and target image respectably. The modification text will be the state of the target image. Hence the system is supposed to retrieve images of the same object as the query image, but with the new state described by text. 



\begin{figure*}
\begin{center}
\includegraphics[width=0.8\linewidth]{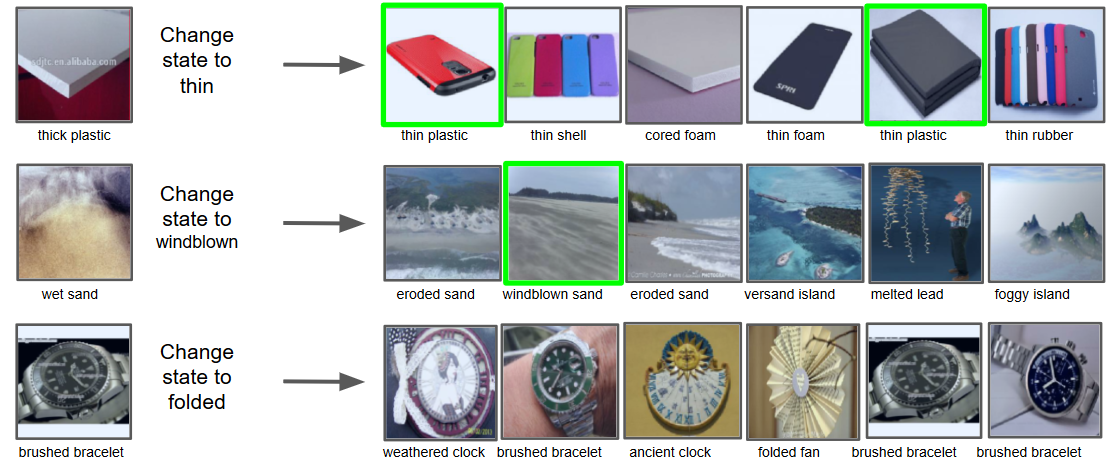}
\end{center}
   \caption{Some retrieval examples on MIT-States.}
\label{fig:mitstatesqual}
\end{figure*}



Some qualitative result is shown in figure \ref{fig:mitstatesqual} and the R@k performance is shown in table \ref{tab:mitstates}. Note that similar types of objects with different states can look drastically different, making the the role of modification text more important than that of query image. Hence on this dataset, the "Text only" baseline outperforms "Image only".

The difference between methods is not too significant at R@1. At R@10, our is slightly better than other baselines.




\begin{comment}


Note that due to the simple nature of image and the composition, it is possible to have an expectation of what the target image would look like. This might not be the case for the other 2 datasets (which have more realistic image and complex/abstract kind of composition).

Today state of the art vision systems are seemingly able to recognize many concepts. To advance their capability of higher level semantic understanding and reasoning, a lot of recent research efforts has been made on manipulation, inference or making arguments based on those concepts. Examples include studying of compositionality \cite{misra2017red, nagarajan2018attributes} and studying of vision plus language problems (captioning or VQA). In this work, through the image retrieval task, we study how to compose image and text.


In a traditional image retrieval system, user query is image based or text based, each has their own advantages and use cases. Image query is good when searching for object/scene at instance level or with specific configuration/appearance that is difficult expressed in text; on the other hand, for a lot of concepts, especially abstract one, it is easier to expressed using language, hence text query is better. Here we consider the use case where users can use both image and text to specify what they look for; this allows them to use an example image as reference and then add additional modification description in text, resulting in a more expressive query. We call this task image retrieval with image text composition query; example is shown in figure \ref{fig:task}.


\begin{figure}[t]
\begin{center}
% \includegraphics[width=0.99\linewidth]{res/intro.png}
\includegraphics[width=0.85\linewidth]{res/intro2.png}
\end{center}
   \caption{Example of image retrieval using image text composition query.}
\label{fig:task}
\end{figure}


Similar to state of the art image retrieval systems, our approach to this task is to learn a deep embedding space, which usually is semantically meaningful. Since composition between image and text is also at high level semantic, it will be performed on this space (rather than, say, the image pixel space).

To learn this compositional visual text embedding, we propose a method of modifying  image representation via residual value. It basically leverages a ResNet block for feature fusion between image and text, with additional weighting and gating so that the network can control how much the image query and the text query contribute to the final composition feature. Our intuition is that it is easier for a deep network to use the query image feature as reference and then inject minor modification described by the text, than to compose a brand new feature, as commonly done in previous works.

Our contributions are: (1) we augment image retrieval with image text composition query and create a new dataset for testing such task, (2) to model the composition, we investigate several baselines and proposed a feature modification via residual value approach, and (3) extensive experiments are performed on our new dataset and 2 other datasets to validate our proposed method.

The rest of the paper is organized as follow: we discuss related works in section 2. The problem formulation and our proposed approach are described in section 3; lastly we show experiments result in section 4 and conclude in section 5.
\end{comment}


\begin{comment}
\lu{do we have ablation studies on $k$?}
\nam{no, the formulation just for unifying the 2 losses we used. we don't have its implemented.}
\lu{something to consider for ablation studies where k = 5, 10, ...}
\nam{not possible unless we redo the implementation and experiments}
\lu{I think you can choose k in the classification case?}
\nam{no, changing k can exponentially change the number of clusters, which is fixed in current implementation. Dealing with exponentially large clusters can be tricky to implement. Might take a while, and risky if we want to go this road.}
\lu{can we at least do a comparison between k=2 and k$\ne 2$}
\nam{we have 2 cases, smallest value k=3, and biggest value k=n+1. The result is previously reported: on CSS & MIT, the first one works the best, on Fashion200k, the second one is better}
\lu{let's include those in ablation studies}
\nam{for the cases that it's not better, I didn't really try to do the whole "experiment" thing, so I have to run those if we want to include them. I can do it once I'm done with the current experiments.}
\lu{ok. I thought you have everything. since you do not have, it is not important then}
\end{comment}



%\begin{figure}[t]
%\begin{center}
%\includegraphics[width=0.7\linewidth]{res/css2.png}
%\end{center}
%   \caption{Example images in our CSS dataset. Each row shows the same scene in 2D and 3D rendered images. \lu{is this useful we have the info in Fig.4 already}}
%\label{fig:css}
%\end{figure}

\section{Identity connection}

The difference between our proposed approach compared to baseline such as concat fusion is having the identity connection contributing to the output feature.
In section 4.2, we show some visualizations to demonstrate the effect of having an identity connection. On the MIT-State dataset, we can show some quantitative effect. Here the retrieved image is considered correct if it has the correct object label (extracted from the image part of the query) and the correct state label (extracted from the text part of the query). Hence in addition to measuring composition retrieval performance, we can also measure correct object or correct state retrieval performance to analyze how well the composition module extract those separate information from each channel of the input query, the result is shown in figure \ref{fig:mitstates_r1_object_state}.

For the concat fusion (and also other baselines that creates new output feature from input), the object, state and together composition performance improves during training as expected. Differently, for our approach, the object retrieval performance is already quite high right at the beginning. This is because the output feature is mostly the query image feature with no modification is yet learned. As training goes, correct object performance is actually compromised to improve the overall correct composition retrieval performance.

We can measure the contribution to the composition feature of the identity connection by computing its magnitude over the sum of all connection's magnitude. It'd start big and then get smaller as the residual connection learns to model the needed modification. In table \ref{tab:identity}, we show that value for each dataset when training converged. It seems that with more realistic images and complex composition, Fashion200k and MIT-States are relying less on the identity connection compared to CSS.



\begin{figure*}
\begin{center}
\includegraphics[width=0.9\linewidth]{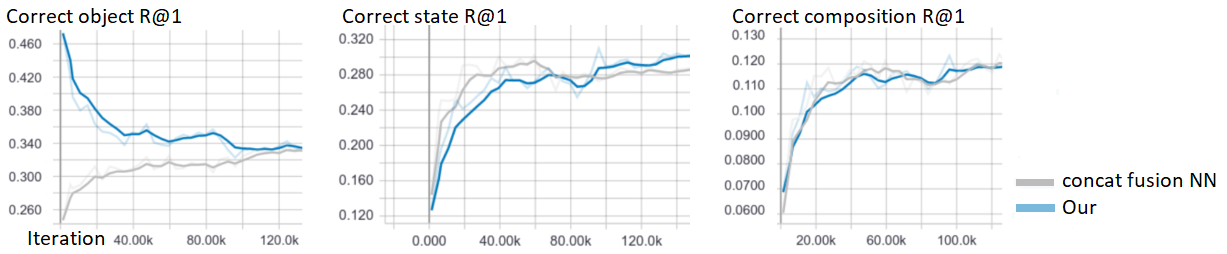}
\end{center}
   \caption{Retrieval performance changing during training on MIT-States.}
\label{fig:mitstates_r1_object_state}
\end{figure*}


\begin{comment}
\begin{table}
\begin{center}
\begin{tabular}{|l|c|}
\hline
Dataset & Identity's contribution \\
\hline\hline
CSS & 62\% \\
Fashion200k  & 20\% \\
MIT-States & 31\% \\
\hline
\end{tabular}
\end{center}
\caption{The average contribution to the composition feature of the identity connection in our approach in each dataset.}
\label{tab:identity}
\end{table}
\end{comment}
